# Supplementary material for: Looking for central tendencies in the conformational freedom of proteins using NMR measurements
Source: arXiv:1602.05953 ancillary file (2016-02-18)
Supplement: Supplementary file 1 [file supplementary.pdf]

# LOOKING FOR CENTRAL TENDENCIES IN THE CONFORMATIONAL FREEDOM OF PROTEINS USING NMR MEASUREMENTS.
—
# SUPPLEMENTARY MATERIAL

FABRIZIO CLARELLI[(1)] AND LUCA SGHERI[(1,*)]

## 1. Introduction

This supplementary material contains some topics which deepens the analysis of the data, but are not strictly necessary for the main paper. In Section 2 we show that the sets of PCS and RDC measurements are almost linearly independent. In Section 3 we show that there is a modification in the simulated distribution due to removal of the positions of the C terminal which are not allowed since they would cause some physical violations. Finally in Section 4 we show why a joint PCS+RDC case does not substantially improve the quality of the solution.

## 2. Linear Independence of RDC and PCS

In this section we analyse the linear independence of RDC and PCS measurements. The simplex algorithm may be run using different sets of data. Let $\bar{d} \in D$ the true unknown probability distribution used to generate some mean RDC and PCS, and let $(R, t)$ be an Euler transformation. Let $p^{rdc}_{\max}(R)$ be the output of the simplex algorithm using the set of RDC alone (note that this does not depend on $t$). Analogously, let $p^{pcs}_{\max}(R, t)$ be the output of the algorithm when using the set of PCS alone. Finally, let $p_{\max}(R, t)$ be the output of the algorithm in the combined PCS+RDC case. The obvious relation between these quantities is the following:

**Property 2.1.** *We have* $p_{\max}(R, t) \leq \min\left(p^{rdc}_{\max}(R), p^{pcs}_{\max}(R, t)\right)$.

*Proof.* The proof is trivial. Let $d \in \hat{\Delta}$ the probability distribution $(1, R, t)$, then from the definition of MAP we have:

$$\Pi(\bar{d}) = p_{\max}(R, t)\Pi(1, R, t) + (1 - p_{\max}(R, t)) \sum_i q_i \Pi(d_i), \tag{1}$$

where $d_i \in \Delta$, $q_i \geq 0$ and $\sum_i q_i = 1$. Then, both the RDC and PCS measurements are separately recovered by this decomposition, so that $p^{rdc}_{\max}(R) \geq p_{\max}(R,t)$, $p^{pcs}_{\max}(R) \geq p_{\max}(R,t)$. □

From the SVD we can also test if the RDC and PCS measurements may be set independently the ones from the others. If this happens, the reverse of Property 2.1 is also true. We recall that

$$V = \{v \in \mathbb{R}^{n_{\text{meas}}} : v = \Pi(d), d \in D\} \tag{2}$$

is the convex set of dimension $N$ embedded in the $\mathbb{R}^{n_{\text{meas}}}$ space determined by the mean RDC and PCS. The matrix $W_N$ is the projection from $\mathbb{R}^{n_{\text{meas}}}$ in $\mathbb{R}^N$.

**Property 2.2.** *Suppose $V = V_{rdc} \times V_{pcs}$, where $V_{rdc}$ and $V_{pcs}$ are convex sets depending respectively only on RDC and PCS measurements. Then*

$$p_{\max}(R,t) = \min\left(p^{rdc}_{\max}(R), p^{pcs}_{\max}(R,t)\right). \tag{3}$$

*Proof.* Take Equation (1) and project in $\mathbb{R}^N$, obtaining

$$\begin{aligned} W_N \Pi(\bar{d}) =& p_{\max}(R,t) W_N \Pi(1,R,t) \\ &+ (1 - p_{\max}(R,t)) W_N \sum_i q_i \Pi(d_i). \end{aligned} \tag{4}$$

The point $W_N \sum_i q_i \Pi(d_i) \in \mathbb{R}^N$ belongs to the boundary of $V$. Since $V = V_{rdc} \times V_{pcs}$ the point also belongs to the boundary of at least one of the two components $V_{rdc}$ and $V_{pcs}$. Then, by taking the projection of (4) on the relevant component, it follows that $p_{\max}(R,t)$ coincides with either $p^{rdc}_{\max}(R)$ or $p^{pcs}_{\max}(R,t)$. □

**Remark:** In order to fulfil the hypothesis of Property 2.2 we performed two tests.

(i) We checked that the projection given by $W_N$ acts separately on the RDC and PCS measurements.
(ii) Given a set of RDC measurements and a set of PCS measurements we checked if the point obtained coupling the separate measurements is anyway a point of $V$. Using the dependence of RDC and PCS on the Euler transformation, a sufficient condition for (ii) is the following. Take any $d_1$ and $d_2$ in $\Delta$, and calculate the RDC from $d_1$ and the PCS from $d_2$. If it is possible to adjust the translations of $d_1$ (thus not changing the RDC) in order to obtain the same PCS measurements obtained with the distribution $d_2$, then (ii) is verified.

**Remark:** If (4) holds, it is not necessary to run the algorithm on the combined RDC+PCS set of measurements. It is sufficient to run the algorithm separately on the RDC and PCS sets and take the minimum of the two results. Moreover, if the answer to the test presented in the previous remark is positive, we may run the algorithm on the RDC to identify rotations with a large MAP, then fix the rotations and determine the translations from the PCS. The choice of the algorithm used to calculate the MAP has been driven by this analysis.

The hypothesis of Property 2.2 is not fulfilled in a strict sense by the measurements. However, the actual data pictures a situation which is very close to the requirements. This property does not depend on the actual measurements, but only on the set of allowable states. We use the SVD of the matrix

$$A = U\Lambda W = (\Pi(\hat{d}_1), \ldots, \Pi(\hat{d}_M)), \qquad (5)$$

where $\hat{d}_i \equiv (R_i, t_i)$, $i = 1, \ldots M$ are random vertices of $V$. The number $M$ should be by far larger than the number of measurements. We set $M = 200000$.

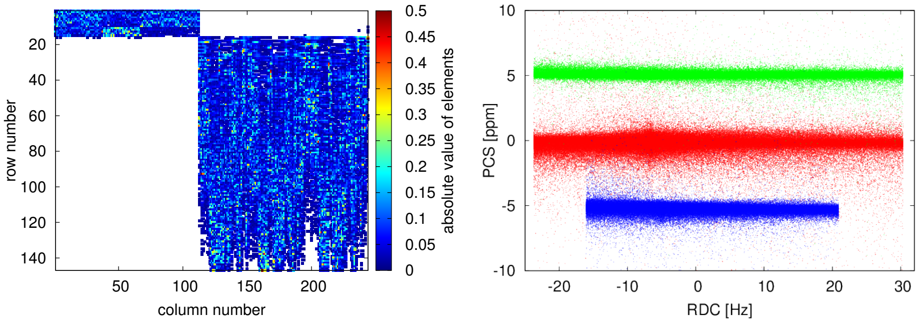


Figure 1. Linear independence of RDC and PCS. Left panel: absolute value of the elements of the projection matrix $W_N$. Right panel: scatter plots of RDC vs PCS. Top: RDC 2 vs PCS 132; Middle: RDC 1 vs PCS 68; Bottom: RDC 50 vs PCS 2. Top and bottom graphs vertically shifted by ±5 ppm for clarity.

The matrix $W_N \subset W$ projects the measurements on the subspace $\mathbb{R}^N$ corresponding to non zero singular values of $A$. A permutation of the matrix $W_N$ is shown in the left panel of Figure 1. The rows are rearranged in order to group the RDC and PCS projection in the $\mathbb{R}^N$ space. Only elements with absolute value larger than 0.01 are shown. The very weak correlation between PCS and RDC is shown

in the right panel, where three example scatter plots are presented. The top and bottom graph are vertically shifted by $\pm 5$ ppm for clarity. Each graph represents the points $(A_{ij_1}, A_{ij_2})$, $i = 1, \ldots, M$, with $j_1$ and $j_2$ indexes corresponding to different RDC and PCS respectively, see equation (5). Note that the top and middle graphs are relative to RDC measured with respect to the same metal ion, so the horizontal range is the same. The bottom graph is relative to a RDC calculated with respect to a different metal ion, hence the different horizontal span. All the scatter plots of this type should be rectangles in order to fulfil test (ii) above. While this is not the case in a strict sense, the shape of the graphs do resemble rectangles.

For comparison we also present in Figure 2 some scatter plots with indexes $j_1$ and $j_2$ both corresponding either to RDC or to PCS. In

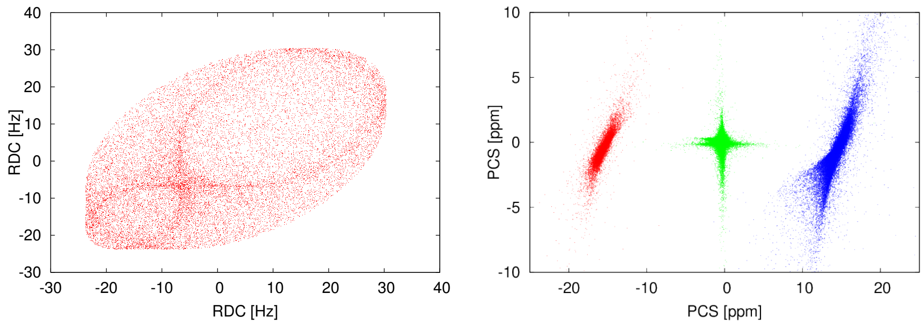


FIGURE 2. Example scatter plots of RDC vs RDC (left panel) and PCS vs PCS (right panel). Left and right plots in right panel horizontally shifted by $\pm 15$ ppm for clarity.

the left panel we present the classic scatter plot of two different RDC. Only one tenth of the points are displayed, in order to show the patterns appearing due to difference in the density of the points. These patterns are related to the behaviour of the trigonometric functions defining the rotation matrices $R_i$ of the distributions $\hat{d}_i = (R_i, t_i)$.

In the right panel we show three scatter plots of PCS versus PCS. The left and right graphs are horizontally shifted by $\pm 15$ ppm for clarity. Note the different behaviour. The left graph represents two PCS relative to the same metal ion for very close atoms, so that there is a heavy linear correlation. The center plot represents the case of PCS with respect to the same metal ion for residuals of the C terminal far apart. Note that in this case the two PCS cannot both assume large values, which are obtained when the residual is close to the metal. Since

the two residuals are far apart, they cannot be both close to the metal. In the right plot of the panel we show the case of PCS referring to different metal ions. In this case the correlation is weaker since it also depends on the relative orientation of the two paramagnetic tensors.

## 3. Asymmetry of the distribution due to violations

As reported in the paper, to simulate the data we use a symmetrical distribution centered in some Euler transformation $(R, t)$. The positions of the conformer which would cause physical violations between atoms of the C and N terminal are excluded from the distribution.

This exclusion has a relevant effect on the distribution when the center position of the C terminal is close to the N terminal. We observe a shift of the transformations with large probability towards positions where the C and N terminals are farther apart. This effect is also noticeable in the $p_{\max}$ results.

In order to check this effect we need to calculate the distance between two conformers $K_1$ and $K_2$, identified by Euler motions $E_i \equiv (R_i, t_i)$, $i = 1, 2$. There are two different approaches to calculate this distance.

The first is to define a mathematical distance between the Euler motions. For the translational part, the Euclidean distance $d_t(t_1, t_2) = \|t_1 - t_2\|$ may be used. For the rotational part the distance may be measured using the quaternion representation, with $d_R(q_1, q_2) = 2 \arccos(|q_1 \cdot q_2|)$. The two formulas may be linearly combined, obtaining

$$d(K_1, K_2) = d_t(t_1, t_2) + c_R d_R(q_1, q_2) \tag{6}$$

for some well chosen constant $c_R$. The main drawback of this definition is that the distance only depends on the angle of rotation of $R_1^t R_2$. Hence this distance does not consider the different effects on the displacement of the C terminal due to a different rotation axis.

The second approach is application-driven. Let $a_1, \ldots a_p$ be the atoms of the backbone of the C terminal, and let $E_i(a_j) \equiv R_i(P_j - t_i)$ be the position of the atom $j$ in the $K_i$ conformer. We then define

$$d(K_1, K_2) = \sqrt{\frac{1}{p} \sum_{j=1}^{p} \|E_1(a_j) - E_2(a_j)\|^2}. \tag{7}$$

Formula (7) is more demanding in terms of computer time, but gives a better perception of the physical distance between positions of the C terminal.

The following test shows that there is a shift in the distribution center due to the simulations. Starting from the central positions $C_k \equiv$

$(R_k, t_k)$, $k = 1 \dots 3$, we simulated the data using the distributions $d_k$ described in the paper. Then we determined the $\hat{C}_k \equiv (\hat{R}_k, \hat{t}_k)$ with the largest $p_{\max}$ using the simplex method procedure also described in the paper. We then calculated the trajectory joining the conformers $C_k$ and $\hat{C}_k$ using slerp [1], and sampled that curve. For each intermediate point $(C_k)_l$ we defined the ball

$$(B_k)_l = \{C : d(C, (C_k)_l) \leq \tau\}, \tag{8}$$

where we selected $\tau = 3$. Finally we generated again the measurements and counted the fraction $(f_k)_l$ of the conformers drawn according to $d_k$ and belonging to $(B_k)_l$. The number $(f_k)_l$ is an estimator of the integral of $d_k$ on $(B_k)_l$. Loosely speaking, $(f_k)_l$ represents the probability of $(C_k)_l$. Figure 3 shows the results.

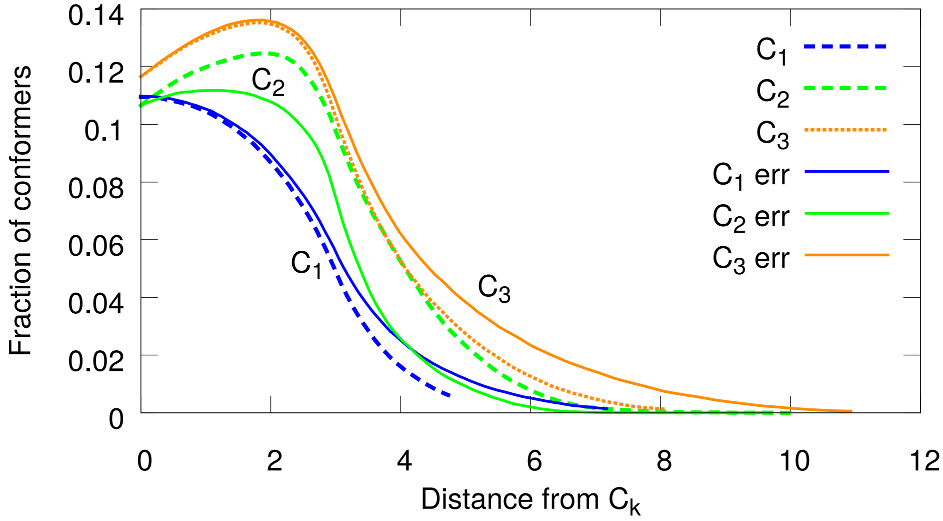


FIGURE 3. Probability of the distributions $d_k$ along a curve joining $C_k$ and $\hat{C}_k$. Dashed lines: cases without error. Solid lines: cases with error.

In the figure, dashed lines represent cases without error, solid lines represent cases with noisy data. Each curve extends up to the $d(C_k, \hat{C}_k)$ horizontal value. A different $\hat{C}_k$ is determined when the error is added, so the dashed and solid lines are sampled along different trajectories. This explains the different behaviour of the solid and dashed line in the case $C_2$. In case $C_1$ (blue lines) the probability is larger in the center of distribution. This is because $C_1$ is far from the N terminal, so there are no positions with physical violations in a neighbourhood of $C_1$. On the other hand in case $C_3$ the probability becomes larger when we move towards the reconstructed position $\hat{C}_3$. This is a consequence

of the fact that $C_3$ is very close to the N terminal, so basically only Euler motions which draw the C terminal away from the N terminal are permitted in that case. The value of the probability distribution $d_3$ is maximal in $C_3$, the center of the distribution. However, when we integrate over a ball, a large fraction of the positions in the ball around $C_3$ are not permitted. The probability distribution decreases when we move along the trajectory towards $\hat{C}_3$. However the conformational freedom widens, so that the fraction of allowed states in the ball increases. As a consequence the integral becomes larger. The case $C_2$ is an intermediate case.

In figure 4 we show the positions of the C terminal in cases $C_2$ and $C_3$ with error. In the right panel the yellow conformer represents $C_3$, center of the probability distribution. The orange conformer represents $\hat{C}_3$, the position recovered from the MAP algorithm. Finally the black conformer is the position $(C_3)_l$ for $l$ corresponding to the maximum of $(f_3)_l$. Analogously in the left panel the pale green conformer is the position $C_2$, the dark green conformer represents $\hat{C}_2$, and the black conformer is the position $(C_2)_l$ for $l$ corresponding to the maximum of $(f_2)_l$.

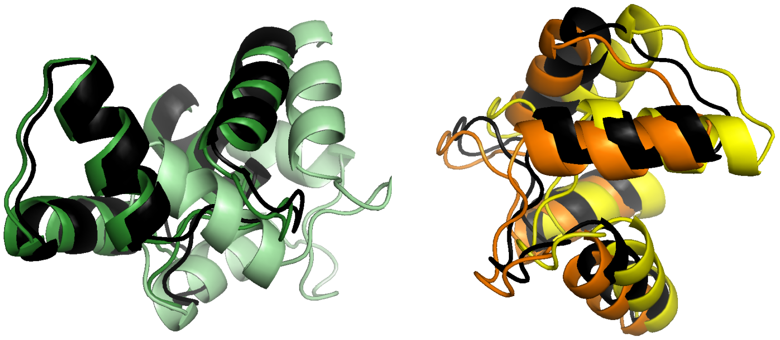

FIGURE 4. The C terminal shown in different positions. Right panel: position $C_3$ *(yellow)*, position $(C_3)_l$ for $l$ corresponding to the maximal $(f_3)_l$ *(black)*, position $\hat{C}_3$ *(orange)*. Left panel: position $C_2$ *(pale green)*, position $(C_2)_l$ for $l$ corresponding to the maximal $(f_2)_l$ *(black)*, position $\hat{C}_2$ *(dark green)*.

## 4. Working together with PCS and RDC

The algorithm described in the paper uses separately RDC and PCS to determine respectively the rotations and translations with large MAP values. The only real benefit found by coupling PCS and RDC is the removal of the ghost cones. Sampling the allowed states with the joint PCS+RDC case does not improve the quality of the solution. To justify this assertion, we report here the results of some tests with noisy data.

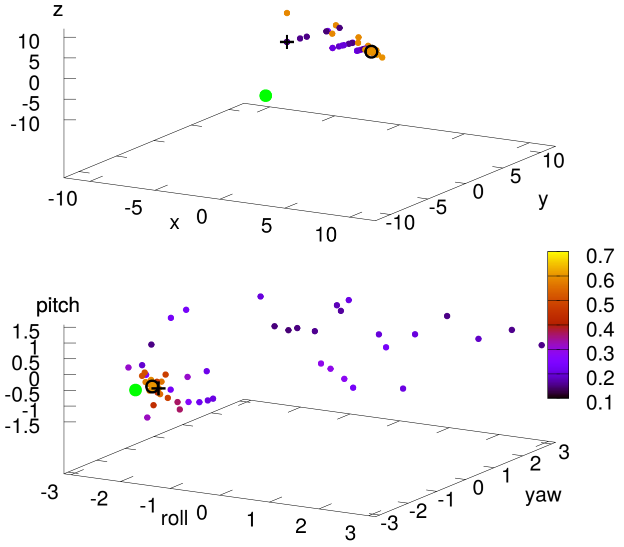


Figure 5. Optimization technique, case $C_2$. Points sampled by the routine. Green dot: model position. Black cross: starting position, i.e. $\hat{C}_2$. Black circle: final position. Top panel: translation. Bottom panel: rotation.

.

Starting from the results $\hat{C}_k$ of the algorithm, we may sample its neighbourhood to refine the results, using the joint PCS+RDC measurements. We have three possibilities.

(1) Changing only the translation. Since the RDC do not depend on the translation, this is equivalent to using only PCS.
(2) Changing only the rotation. While we get a slightly different conformer, its orientation is on average no better than the one of $\hat{C}_k$. This is due to the fact that the PCS values are biased by the error on the translation, so that their contribution is not a real advantage.

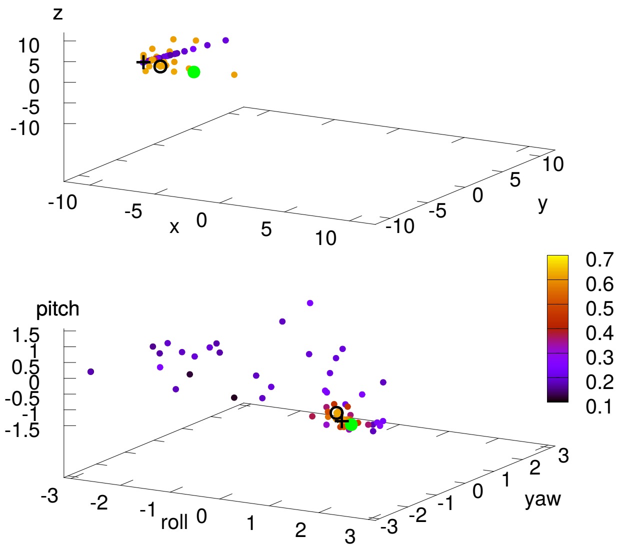


FIGURE 6. Optimization technique, case $C_3$. Points sampled by the routine. Green dot: model position. Black cross: starting position, i.e. $\hat{C}_3$. Black circle: final position. Top panel: translation. Bottom panel: rotation.

.

(3) Changing both the rotation and the translation. The results of this attempt are reported below.

In order to refine $\hat{C}_k$ we implemented a maximization routine using MAP as a merit function, and a polytope algorithm.

In figure 5 we show the points sampled by the optimization routine in case $C_2$, the top panel referring to the translation and the bottom panel to the rotation. The green dots mark the position of the model. The black crosses show the starting point for the routine, i.e. the position of $\hat{C}_2$, while the black circles mark the output of the routine. Figure 6 shows the same information for case $C_3$.

We note that the final rotation does not change substantially with respect to the starting position. On the other hand, the translation approaches the correct value in case $C_2$ but worsen in case $C_3$. This is due to the fact that the MAP value is dominated by the orientation, so the translational part may assume basically any value without influencing the merit function. Thus the final translation determined by the optimization routine is simply the one attached to the rotation having the largest MAP value.

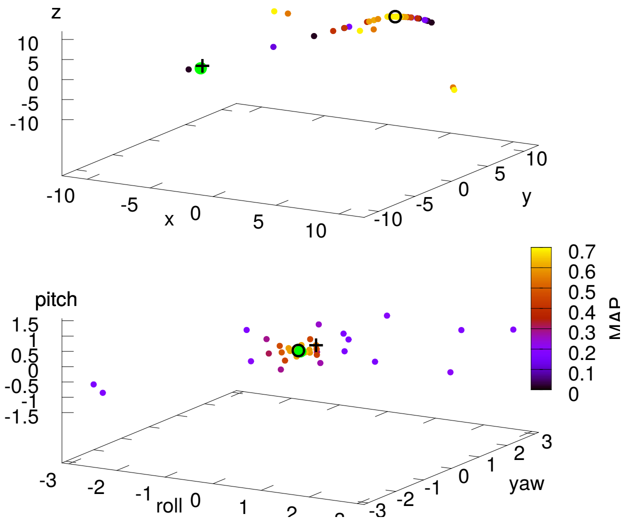


Figure 7. Optimization technique, case $C_1$ with large incertitude on the initial guess. Points sampled by the routine. Green dot: model position. Black cross: starting position, i.e. $\hat{C}_1$. Black circle: final position. Top panel: translation. Bottom panel: rotation.

.

A further experiment proves this assertion. We took the exact values of the measurements in case $C_1$, where the error of the reconstructed conformer from the algorithm is minimal. Then we used a large value for the incertitude of the initial guess, thus permitting the polytope algorithm to sample a large zone of the allowed states of the conformer. In Figure 7 we show the results. We note that, even if the initial translation is rather close to the correct value, the final value gets drifted away.

Thus our conclusion is that the joint PCS+RDC case is not really an advantage. On average a slightly better result can be obtained for the rotational part, but the translational part suffers from the weak dependence of the PCS.

## References

[1] Shoemaker, K 1985 Animating Rotation with Quaternion Curves, *SIGGRAPH '85*, San Francisco.

(1)Istituto per le Applicazioni del Calcolo (CNR), sede di Firenze, Via Madonna del Piano, 10, 50019 Sesto Fiorentino (FI), Italy
*E-mail address*: *l.sgheri@iac.cnr.it
